# Supplementary material for: FuzzCoder: Byte-level Fuzzing Test via Large Language Model
Source: arXiv:2409.01944 source file (2024-09-03)
Supplement: Supplementary file 1 [file Appendix.tex]

\appendix

\appendix

\section{Detailed Results}
